# Supplementary material for: Multiscale Physics-Informed Neural Networks for the Inverse Design of Hyperuniform Optical Materials
Source: arXiv:2405.07878 ancillary file (2024-11-30)
Supplement: Supplementary file 1 [file Hyperuniform_SI_arXiv.pdf]

# **Supporting Information for**
Multiscale Physics-Informed Neural Networks for the Inverse Design of Hyperuniform Optical Materials.

Roberto Riganti, Yilin Zhu, Wei Cai, Salvatore Torquato, and Luca Dal Negro

Corresponding author: Luca Dal Negro
Email: dalnegro@bu.edu

**This PDF file includes:**

Figures S1 to S10
Table S1

**Fig. S1.** $\boldsymbol{S(k)}$ plot for SHU N=396, $\boldsymbol{\chi = 0.5}$.

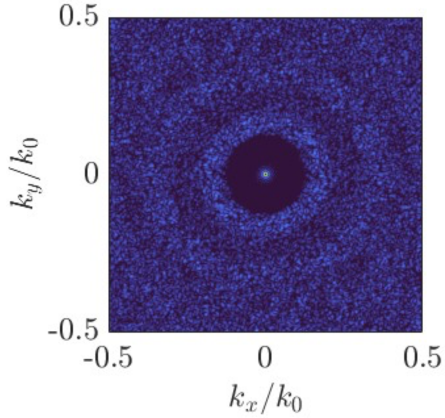

**Fig. S2.** The top two panels show the SHU array and $\boldsymbol{S}(\boldsymbol{k})$ plot with N=663 particles, $\chi = \mathbf{0.3}$. The bottom two panels show the UR array and $\boldsymbol{S}(\boldsymbol{k})$ plot with N=661 particles. These structures were employed in Sections III.A and III.C of the main text. (Pillar size not drawn to scale).

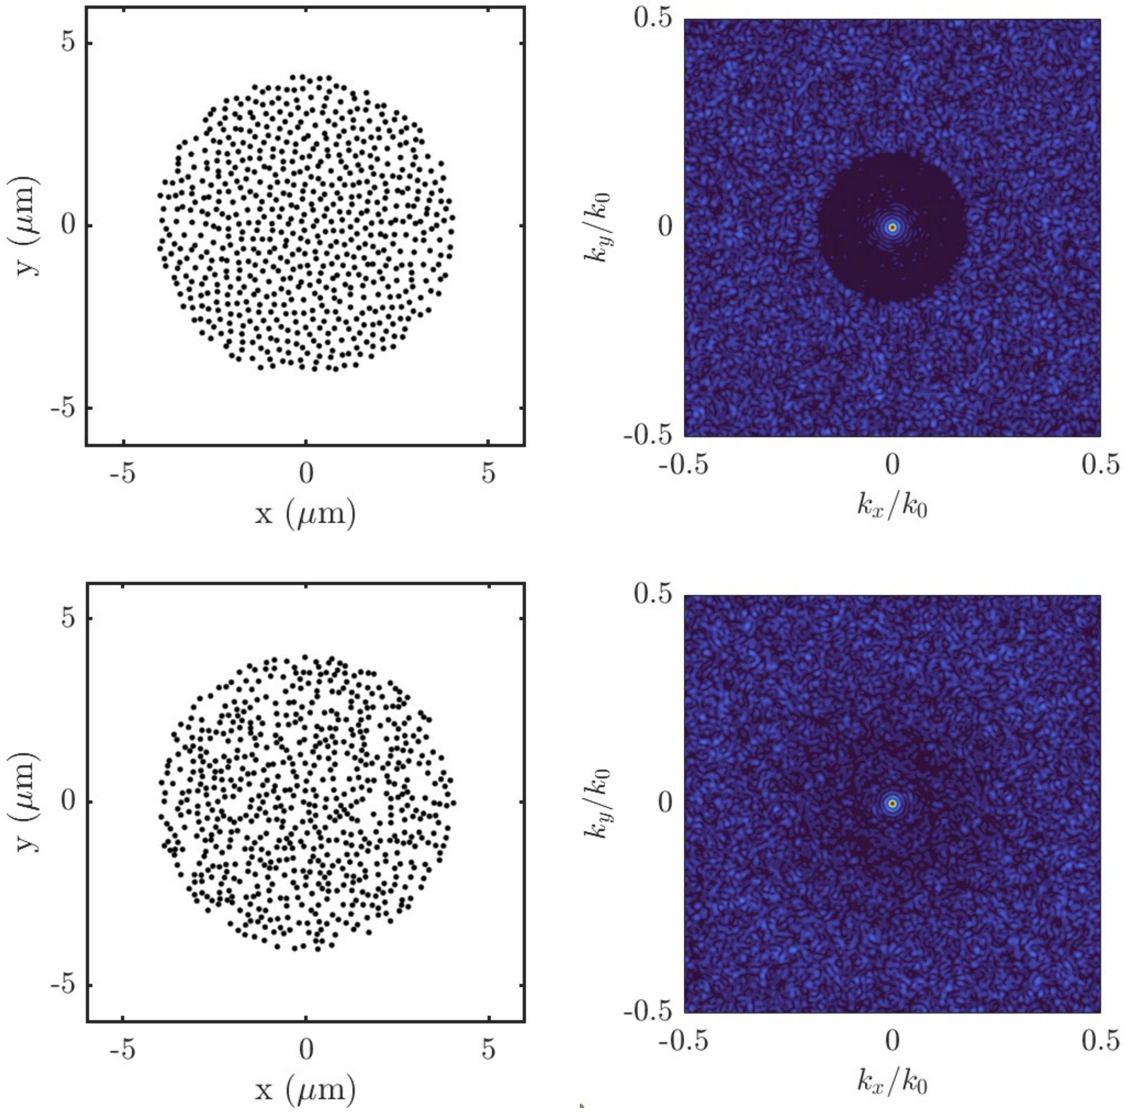

**Fig. S3.** Real part of the electromagnetic fields utilized for the inverse training dataset of the Mscale/single-scale and SHU/Poisson comparison in the main text, namely Sections III.A and III.C. The imaginary part of the electromagnetic field can be provided upon request.

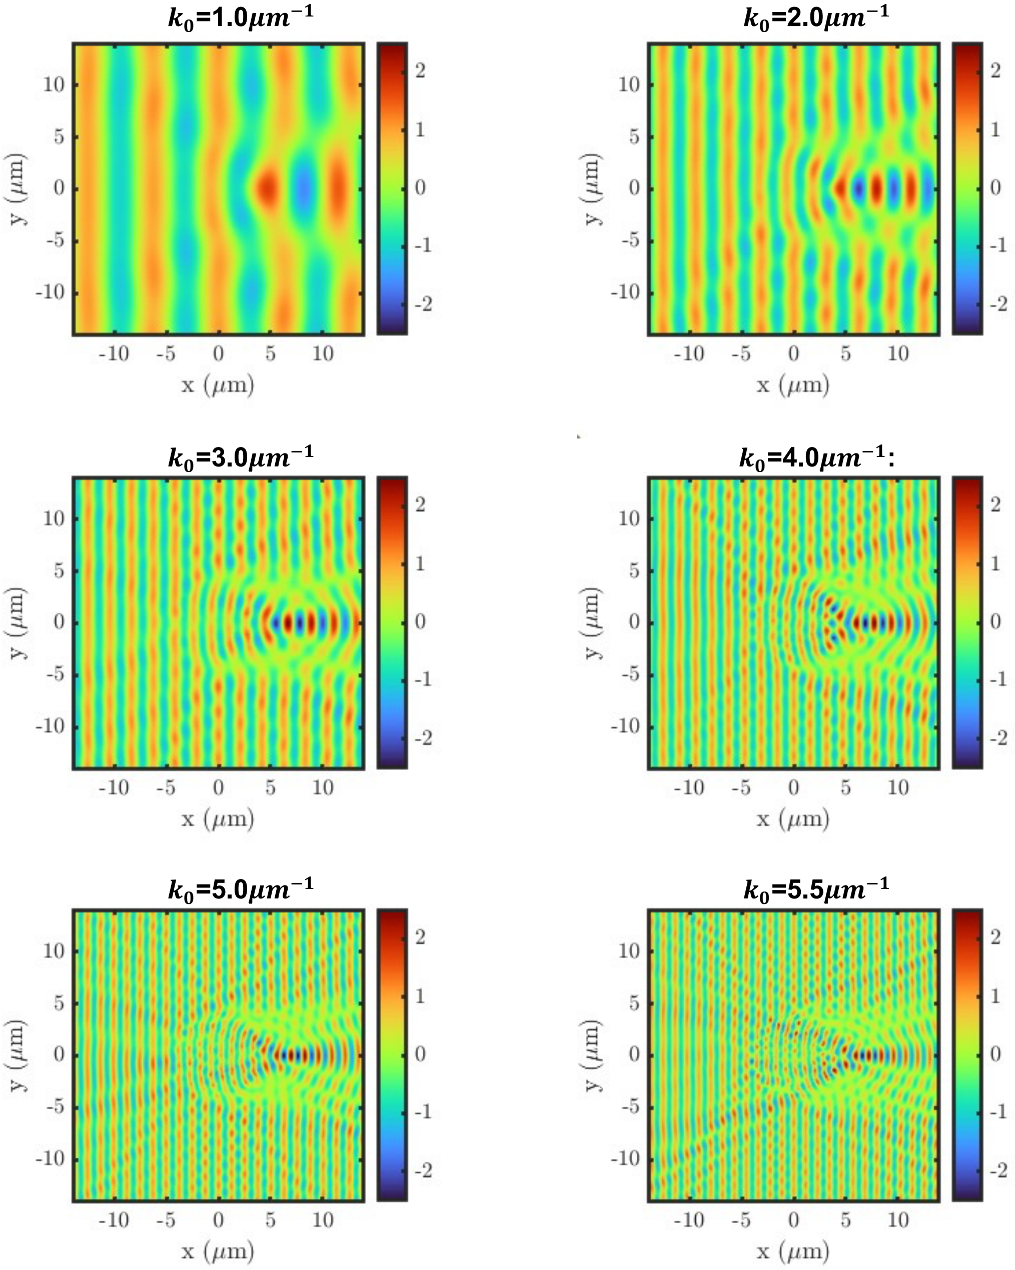

**Fig. S4.** Comparison between the MscalePINN homogenized $\langle \boldsymbol{Re}[\hat{\boldsymbol{\epsilon}}(\boldsymbol{x},\boldsymbol{y})]\rangle$ for the Poisson and SHU structures including all $\boldsymbol{k}$ values. Already at $\boldsymbol{k_0} = \mathbf{3.0}\boldsymbol{\mu m^{-1}}$, the MscalePINN struggles to retrieve a homogeneous effective medium. However, the error on the inhomogeneous retrieved medium is below 5%. For $\boldsymbol{k_0} = \mathbf{5.0}\boldsymbol{\mu m^{-1}}$, MscalePINN fails to retrieve an effective medium with $\boldsymbol{L^2}$ error below 17% for the Poisson structure, and for $\boldsymbol{k_0} = \mathbf{5.5}\boldsymbol{\mu m^{-1}}$, we could not train any configuration of MscalePINN to retrieve a physical value of $\hat{\boldsymbol{\epsilon}}(\boldsymbol{x},\boldsymbol{y})$. For the SHU structure, however, we display homogeneity and high accuracy in the retrieve effective medium until $\boldsymbol{k_0} = \mathbf{5.0}\boldsymbol{\mu m^{-1}}$, which is close to the end of the predicted transparency region.

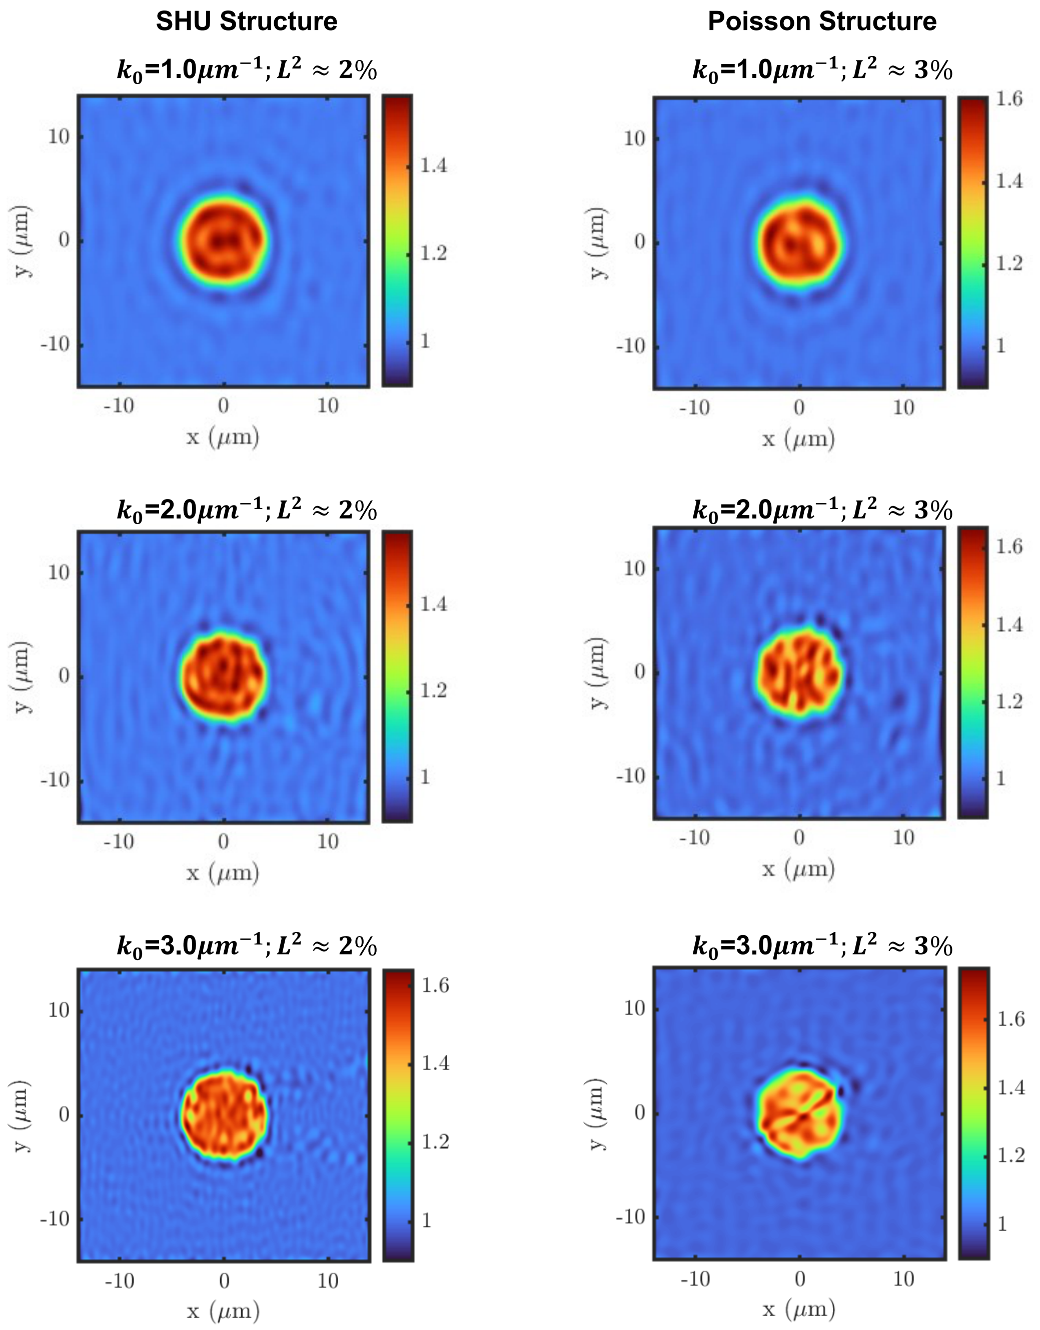

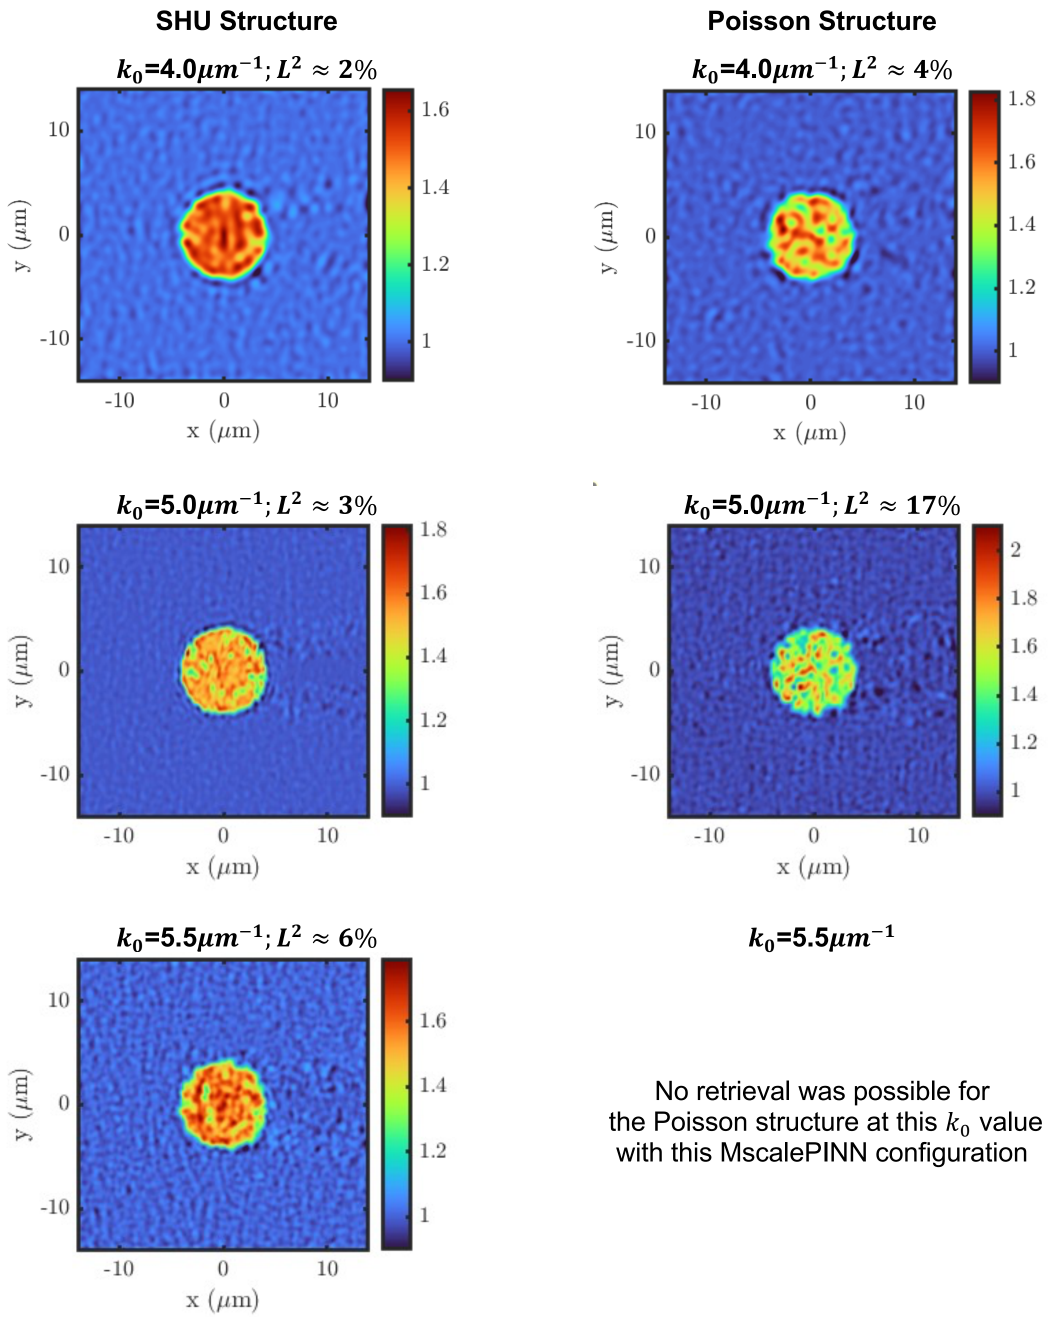


Where the error is given by:

$$L^2 = \frac{\sum_{\mathcal{N}_i} \left| x_p - x_{obs} \right|^2}{\sum_{\mathcal{N}_i} \left| x_{obs} \right|^2}$$

$\mathcal{N}_i$ denotes the residual points for the complex field observations.

**Fig. S5.** Below we display the spread of the real part of $\hat{\epsilon}(\boldsymbol{x}, \boldsymbol{y}; \boldsymbol{k})$ retrieved by MscalePINNs for the same structures from Fig.2 and Fig.4 of the main text for both the Poisson and SHU structure.

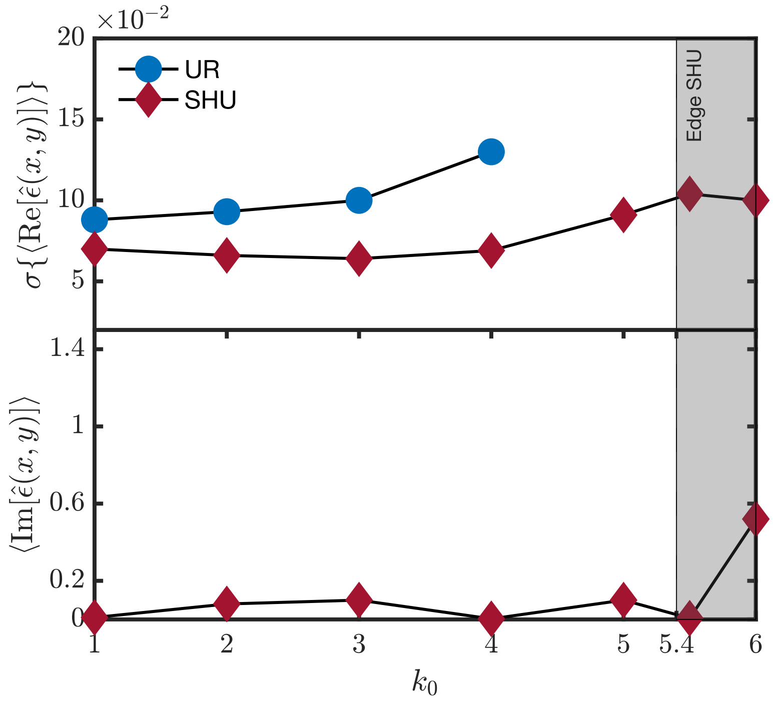


The investigated range of wavenumber $\boldsymbol{k_0}$ corresponds to a ratio of $\frac{\langle d \rangle}{\lambda} = \mathbf{0.034}$ for the longest wavelength and $\frac{\langle d \rangle}{\lambda} = \mathbf{0.19}$ for the shortest wavelength. Despite achieving high accuracy for both structures at values below and including $\mathbf{4.0\mu m^{-1}}$, the MscalePINNs failed to retrieve a localized effective medium for the Poisson structures at higher $\boldsymbol{k}$-vectors.

In contrast, MscalePINNs retrieved a highly accurate homogenized $\hat{\epsilon}(\boldsymbol{x}, \boldsymbol{y}; \boldsymbol{k})$ until the predicted threshold for SHU structures of $\boldsymbol{k_0} \approx \mathbf{5.5\mu m^{-1}}$, with an $\boldsymbol{L^2}$ error of 6%. Beyond this value, displayed by the grey shaded region, MscalePINNs could not retrieve an effective medium for the SHU arrays as well. In this figure, we have included the MscalePINN's prediction based on the single realization beyond the $\boldsymbol{k_0}$ critical value, where the $\boldsymbol{L^2}$ error was much higher with a value of 24%. We also note that for the SHU array, the real part of $\hat{\epsilon}(\boldsymbol{x}, \boldsymbol{y}; \boldsymbol{k})$ becomes less homogeneous as we approach the edge of the predicted transparency region. In this case, the MscalePINN continues to accurately retrieve an effective, albeit inhomogeneous, medium until the predicted edge of $\boldsymbol{k_0} = \mathbf{5.5\mu m^{-1}}$.

**Fig. S6.** $\boldsymbol{S(k)}$ plots of four $\boldsymbol{\chi = 0.3}$ SHU structures with N=299, 633, 1002, and 1553, respectively. This figure shows that, even for $\boldsymbol{N \to 300}$, the stealthy patterns are evident. (Pillar size not drawn to scale).

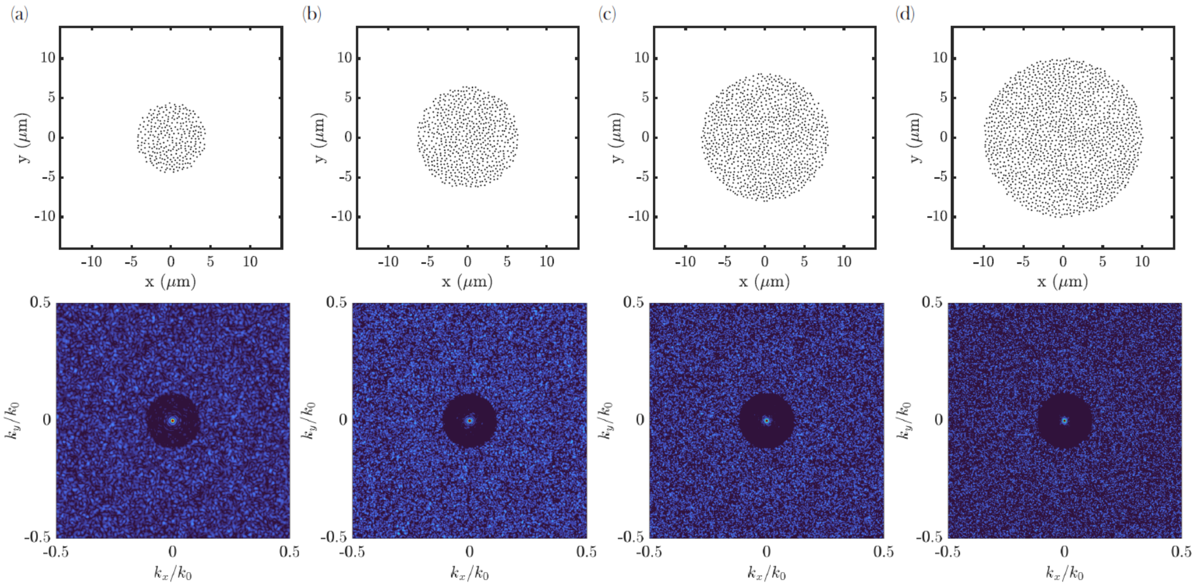

**Fig. S7.** $\boldsymbol{S}(\boldsymbol{k})$ plot for SHU N=236, $\boldsymbol{\chi} = \mathbf{0.5}$.

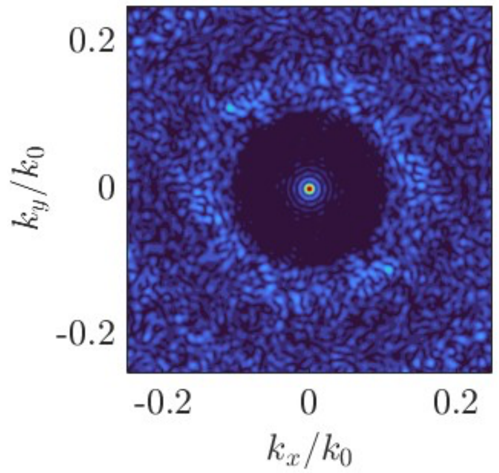

**Fig. S8.** Real part of the electric field used for the angular independence study in Fig.6 of the main text.

**0° incidence**

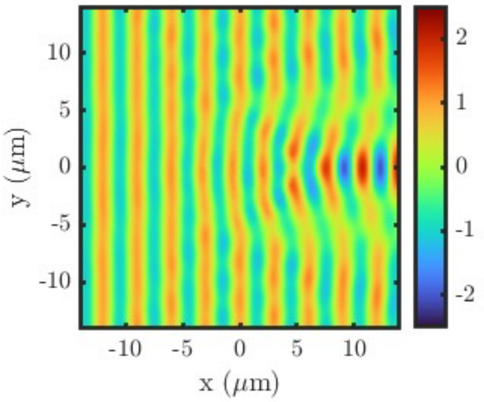


**45° incidence:**

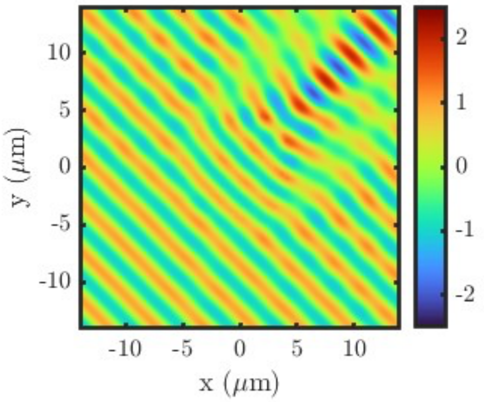


**-30° incidence:**

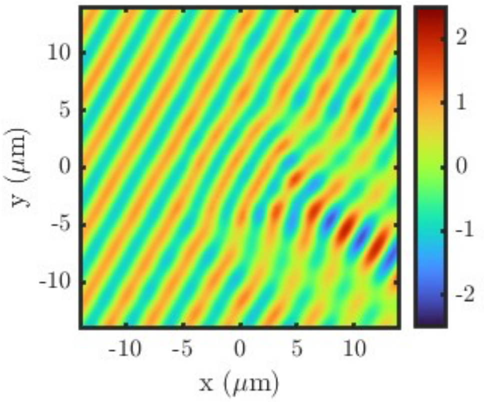

**Fig. S9.** Retrieved binarized structure from section 3.7 of the main text, where $\boldsymbol{\lambda} = \mathbf{2.0\mu m}$. This is the final output of the MscalePINN before we apply the $\boldsymbol{\Theta}$ function from Eq (27) in post-processing.

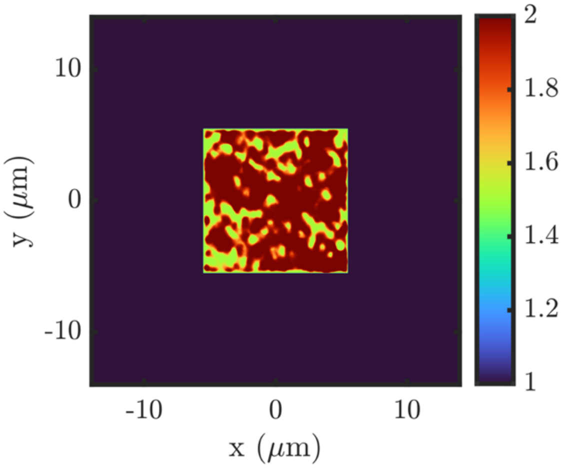


Representative comparison between the real part of the electromagnetic field employed during training (left) and the real part of the electromagnetic field obtained via a forward simulation on the structure above (right). The total $L^2$ error on the complex field was 3%.

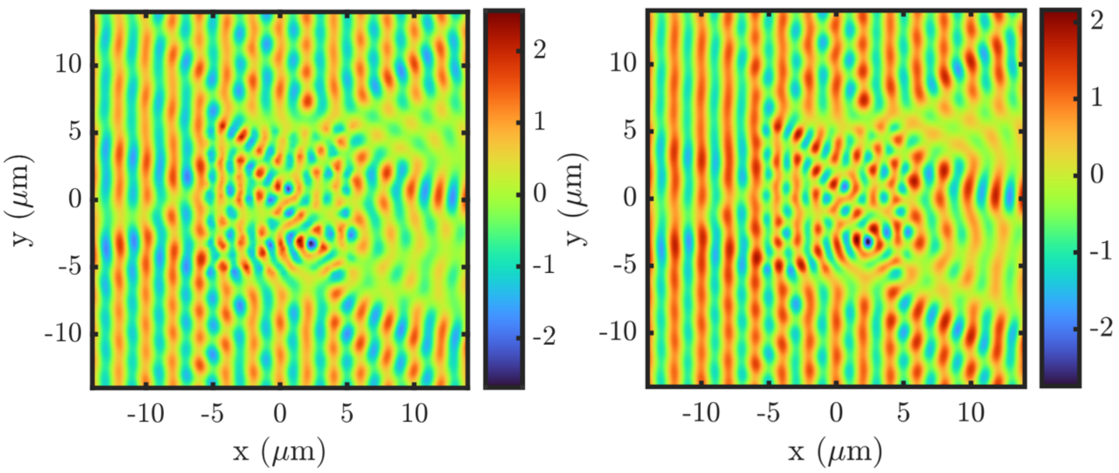

**Fig. S10.** Real and imaginary part of the electric field used to train MscalePINN to retrieve the focusing effective medium shown in Fig. 8(e) of the main text. Here, $\lambda = 1.0\mu\text{m}$.

**Re**$\{\boldsymbol{E_z}\}$**:**

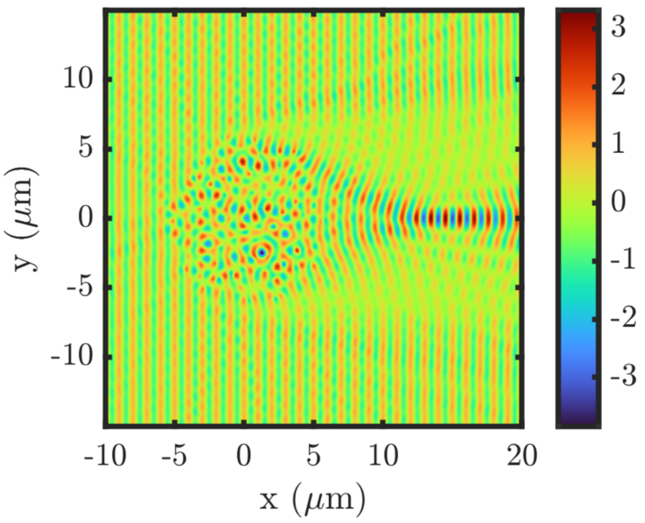


**Im**$\{\boldsymbol{E_z}\}$**:**

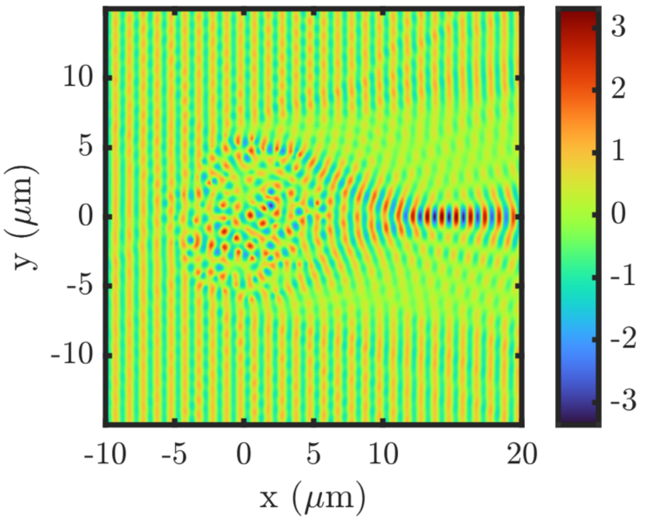

**Table S1.** MscalePINN training information in order of appearance.

For the MscalePINN training we employed the ADAM optimizer with a piecewise constant learning rate decay. The learning rate varied from a starting value of 1e-2 to a final value of 1e-5, with one order of magnitude decrease every 25% of the total epoch count. For all the simulations we employed the sin(x) activation function, and we trained the network on 32,768 ($\mathbf{2^{15}}$) collocation points in the interior and 40,000 points for the inverse FEM field dataset. Each problem treated required some tuning of hyperparameters such as network scales and number of epochs, which are listed below.

**Problem-specific hyperparameters:**

| Structure | Epochs | Scales | Scale factors | Layers/ scale | Neurons /layer | Loss value |
|---|---|---|---|---|---|---|
| SHU N=663, k=1.0 | 40,000 | 4 | {1, 2, 4, 8} | 4 | 64 | 8e-5 |
| SHU N=663, k=2.0 (Fig. 2a) | 40,000 | 4 | {1, 2, 4, 8} | 4 | 64 | 9e-4 |
| SHU N=663, k=2.0 (Fig. 2b) | 40,000 | 1 | {1} | 4 | 64 | 5e-4 |
| SHU N=663, k=3.0 (Fig. 4a) | 40,000 | 4 | {1, 2, 4, 8} | 4 | 64 | 2e-3 |
| SHU N=663, k=4.0 (Fig. 2c) | 40,000 | 10 | {1, 2, …, 9, 10} | 2 | 64 | 1e-2 |
| SHU N=663, k=4.0 (Fig. 2d) | 40,000 | 1 | {1} | 8 | 64 | 0.25 |
| SHU N=663, k=5.0 (Fig. 4c) | 150,000 | 10 | {1, 2, …, 9, 10} | 4 | 64 | 8e-3 |
| SHU N=663, k=5.5 (Fig. 2e) | 100,000 | 15 | {1, 2, …, 14, 15} | 2 | 64 | 4e-2 |
| SHU N=663, k=5.5 (Fig. 2f) | 150,000 | 1 | {1} | 8 | 64 | 1.14 |
| SHU N=663, k=6.0 | 100,000 | 15 | {1, 2, …, 14, 15} | 2 | 64 | 8e-2 |
| UR N=661, k=1.0 | 40,000 | 4 | {1, 2, 4, 8} | 4 | 64 | 5e-4 |
| UR N=661, k=2.0 | 40,000 | 4 | {1, 2, 4, 8} | 4 | 64 | 3e-3 |
| UR N=661, k=3.0 (Fig. 4b) | 40,000 | 4 | {1, 2, 4, 8} | 4 | 64 | 1e-2 |
| UR N=661, k=4.0 | 40,000 | 10 | {1, 2, …, 9, 10} | 2 | 64 | 2e-2 |
| UR N=661, k=5.0 (Fig. 4d) | 100,000 | 10 | {1, 2, …, 9, 10} | 4 | 64 | 2e-2 |
| UR N=661, k=5.5 | 150,000 | 4 | {1, 2, 4, 8} | 4 | 64 | 7e-1 |
| SHU N=396 (Fig. 3) | 40,000 | 4 | {1, 2, 4, 8} | 4 | 64 | 1e-3 |
| SHU N=299 (Fig. 5a) | 40,000 | 4 | {1, 2, 4, 8} | 2 | 64 | 2e-4 |
| SHU N=633 (Fig. 5b) | 40,000 | 4 | {1, 2, 4, 8} | 2 | 64 | 2e-4 |
| SHU N=1002 (Fig. 5c) | 40,000 | 4 | {1, 2, 4, 8} | 2 | 64 | 1e-2 |
| SHU N=1553 (Fig. 5d) | 40,000 | 4 | {1, 2, 4, 8} | 2 | 64 | 2e-3 |
| SHU N=236, $\theta = 0°$ (Fig. 6b) | 40,000 | 4 | {1, 2, 4, 8} | 4 | 64 | 8e-4 |
| SHU N=236, $\theta = -30°$ (Fig. 6c) | 40,000 | 4 | {1, 2, 4, 8} | 4 | 64 | 8e-4 |
| SHU N=236, $\theta = 45°$ (Fig. 6d) | 40,000 | 4 | {1, 2, 4, 8} | 4 | 64 | 1e-3 |
| SHU N=705 (Fig. 7) | 40,000 | 4 | {1, 2, 4, 8} | 4 | 64 | 1e-4 |
| SHU square (Fig. 8a) | 20,000 | 5 | {1, 2, 4, 8, 10} | 2 | 64 | 8e-3 |
| SHU square (Fig. 8c) | 100,000 | 7 | {1, 2, 4, 8, 10, 14, 18} | 2 | 64 | 1e-2 |
| Focusing (Fig. 8e) | 100,000 | 12 | {3.14, 5, 6.28, 7, 8, 9, 10, 11, 12, 13, 15, 20} | 2 | 64 | 2e-2 |
